# Supplementary material for: On the nature of the glass transition in atomistic models of glass formers
Source: arXiv:1804.03769 ancillary file (2018-04-12)
Supplement: Supplementary file 1 [file Supplemental_Material.pdf]

# On the nature of the glass transition in atomistic models of glass formers: Supplemental Material

Alexander Hudson and Kranthi K. Mandadapu
*Department of Chemical Engineering, University of California, Berkeley, CA 94720, USA and Lawrence Berkeley National Laboratory, Berkeley, CA 94720, USA*

In this Supplemental Material, we present the results of many additional calculations probing the spatial distribution of particles that displace over short observation times. These results support the conclusion reached in the main text that this distribution is ideal-gas-like, both above and below the glass transition temperature $T_g$, and together they confirm that the results presented in the main text in figure 4 are not simply the result of a particular choice of observation time $t$, cutoff distance $a$, or indicator function $h_i(t, a)$.

## I. CHOICE OF OBSERVATION TIME AND DISTANCE CUTOFF

In figures 1–3, we plot $\ln p(\ell^3)$ against $\ell^3$ (ala figure 4 in the main text) for the Kob-Andersen model when subjected to cooling at various rates. Figure 1 shows results for the slowest cooling rate $\nu$, while figures 2 and 3 show results for intermediate ($10\nu$) and fast ($100\nu$) cooling rates, respectively. In each figure, we show six separate plots, each corresponding to different choices of the parameters $t$, the observation time, and $a$, the cutoff distance in the indicator function $h_i(t, a)$ defined in equation 14 of the main text. The observation time varies from $10-1000\tau_{LJ}$ and $a/\sigma \in \{0.6, 1.0\}$.

Increasing the observation time allows more excitations to become manifest through particle displacements. The latter occur stochastically and, as figure 3 of the main text suggests, at a temperature-dependent rate. As a result, fixing the observation time at some small value (e.g., on the order of an instanton time, or $t \approx 10\tau_{LJ}$) ensures that at very low temperatures $T \ll T_g$, we sample only a very small fraction of the excitations still present in the system. This "sub-sampling" of excitations decreases the observed signal and also effectively convolves the "real" distribution $p(\ell)$ with an ideal-gas-like (i.e., exponential) distribution. Furthermore, at such low temperatures the aging process proceeds slowly, so that the underlying distribution of excitations ought to remain essentially fixed as long as $t \ll \tau$ at that temperature. At higher temperatures, increasing the observation time is both less necessary (because displacements occur more rapidly) and more problematic (due to rapid aging). Consequently, we only show results for larger observation times when $\tau > \tau$ at that temperature.

Despite variations in $t$ and $a$, however, the results in figures 1–3 are qualitatively unchanged from the results shown in figure 4 of the main text. As expected, increasing $t$ and decreasing $a$ increase the number of observed displacements, which manifests as a steeper slope in plots of $\ln p(\ell^3)$. Nonetheless, in all cases the distributions are consistent with the pictured described in the main text: beyond a few particle diameters, particle displacements are uncorrelated. In the main text we showed this result for the slowest cooling rate studied; in figures 2 and 3 of this SM, we show that these results are qualitatively unchanged for faster cooling rates.

## II. CHOICE OF MODEL

In figure 4 we show the spatial distribution of excitations for the Wahnström model [1], another popular model of glass-forming liquids, for two different cooling rates. The results are similar to those found in figures 1–3 for the Kob-Andersen model. The only noticeable difference is the greater enhancement of probability at low $\ell$ compared to the KA model; however, beyond a few particle diameters, the distributions become remarkably exponential, just as for the KA model. The results in figure 4 suggest that the results presented in the main text (and this SM) are not specific to the choice of model.

## III. CHOICE OF DYNAMIC INDICATOR OF UNDERLYING EXCITATIONS

The results in the main text and figures 1–3 of this SM show that the spatial distribution of displacing particles remains remarkably exponential, or ideal-gas-like, even for $T \ll T_g$, in contrast to our expectations based on prior East model results. Specifically, particles satisfying $h_i(t, a) = 1$, where

$$h_i(t, a) \equiv \Theta\left(|\bar{\mathbf{r}}_i(t) - \bar{\mathbf{r}}_i(0)| - a\right) \quad (1)$$

is a dynamic order parameter indicating whether particle $i$ has displaced at least a distance $a$ in an observation time $t$, are uncorrelated for a wide variety of choices of $a$, $t$, and the cooling rate.

One possible explanation for this discrepancy is that the function in equation 1 is a poor indicator of underlying excitations. In using it, we have assumed that any changes in inherent structure occurring on a length-scale $\sim\sigma$ correspond to facilitated dynamics and are thus directly connected to the presence and rearrangement of underlying excitations. This assumption could be invalid if the atomistic analogue of facilitated dynamics in KCMs is more complex than simple single-particle displacements. We might imagine that some of the changes in inherent structure captured by the function in equation 1 do not lead to a significant local rearrangement of particles, nor do they facilitate rearrangements at later times, and are therefore irrelevant to structural relaxation. By including these irrelevant motions, we obscure the true spatial distribution of excitations when computing $p(\ell)$. In particular, if these irrelevant motions occur at random throughout the system, we would expect $p(\ell)$ to appear more ideal-gas-like than the true distribution.

Assuming this explanation is correct, the indicator function in equation 1 must be replaced with another function capable of distinguishing relevant dynamics from irrelevant dynamics. Constructing such a function requires physical insight into which changes in inherent structure are important, i.e., what kinds of particle displacements actually lead to *facilitation* and eventual structural relaxation. One possibility is that facilitated dynamics is represented by *strings* of particles that move along quasi-one-dimensional paths. Previous work [3, 4] has shown that dynamics in supercooled liquids becomes increasingly string-like as temperature is lowered, and the physical picture of this string-like motion, with particles filling the voids left by their displacing neighbors, is consistent with our intuition about facilitation [2].

To test the possibility that $p(\ell^3)$ will display the expected non-exponential behavior for $T < T_g$ if we use string-like motion as our proxy for excitations, rather than simple displacements as in equation 1, we construct a pairwise indicator variable $h^s_{ij}(t,a)$ that detects whether particles $i$ and $j$ participate in a string-like motion in an observation time $t$:

$$h^s_{ij}(t,a) \equiv \Theta\left(a - \min\left\{d_{ij}(t), d_{ji}(t)\right\}\right). \quad (2)$$

Here, $d_{ij}(t) \equiv |\bar{\mathbf{r}}_i(t) - \bar{\mathbf{r}}_j(0)|$ gives the distance between particle $i$ at time $t$ and particle $j$'s initial position. The function $h^s_{ij}(t,a)$ indicates whether one of particles $i$ or $j$ assumes the original position of the other particle in an observation time $t$, within a tolerance specified by the parameter $a$. This definition is similar in spirit to the one in reference [3]. We then define a string as a set of particles connected by this string-like motion. Concretely, if $S$ is a string, then $i \in S$ and $j \in S$ if and only if there exists a sequence of particles $k_1, k_2, \ldots, k_n$, also members of $S$, such that

$$h^s_{ik_1} h^s_{k_1 k_2} \cdots h^s_{k_{n-1}k_n} h^s_{k_n j} = 1.$$

This definition can be understood by imagining that we can reach particle $i$ from particle $j$, or vice versa, by following a sequence of displacements, which is consistent with our intuitive notion of string-like motion.

With mobile particles identified and clustered into strings according to the preceding definitions, we can compute the spatial distribution of the strings, with the position of a string $S$ given by the mean position of its particles:

$$\mathbf{r}(S) \equiv \frac{1}{|S|} \sum_{i \in S} \bar{\mathbf{r}}_i(0).$$

In figure 5 we show nearest-neighbor distributions of strings for the same set of observation times and temperatures as in figures 1–3, for the Kob-Andersen model subjected to our slowest cooling rate. The left column shows the results for $a = 0.6$ (the choice in reference [3]), while the right column shows the results for the more stringent choice $a = 0.4$. The results remain remarkably exponential, despite employing a much more complex definition of excitation dynamics than in the main text.

The results in figures 1–3 and 5 suggest that the ideal-gas-like distribution that we have repeatedly found is a robust result, insensitive not only to the particular choices of parameters used to detect excitations but also to the very definition of excitation dynamics. Although we cannot entirely rule out the possibility that the "true" excitation dynamics still eludes us, and that a more faithful indicator would yield a non-exponential distribution of inter-excitations distances, we believe it more likely that excitations, as they have traditionally been understood, remain spatially uncorrelated *even as the liquid falls out of equilibrium.* Reconciling the latter observation with our intuition from hierarchical models, such as the East model or the triangular plaquette model [5], is left to future work.

[1] G. Wahnström, Physical Review A **44**, 3752 (1991).
[2] A. S. Keys, L. O. Hedges, J. P. Garrahan, S. C. Glotzer, and D. Chandler, Physical Review X **1**, 021013 (2011).

[3] C. Donati, J. F. Douglas, W. Kob, S. J. Plimpton, P. H. Poole, and S. C. Glotzer, Physical Review Letters **80**, 2238 (1998).
[4] Y. Gebremichael, M. Vogel, and S. C. Glotzer, The Journal of Chemical Physics **120**, 4415 (2004).
[5] J. P. Garrahan, Journal of Physics: Condensed Matter **14**, 1571 (2002).

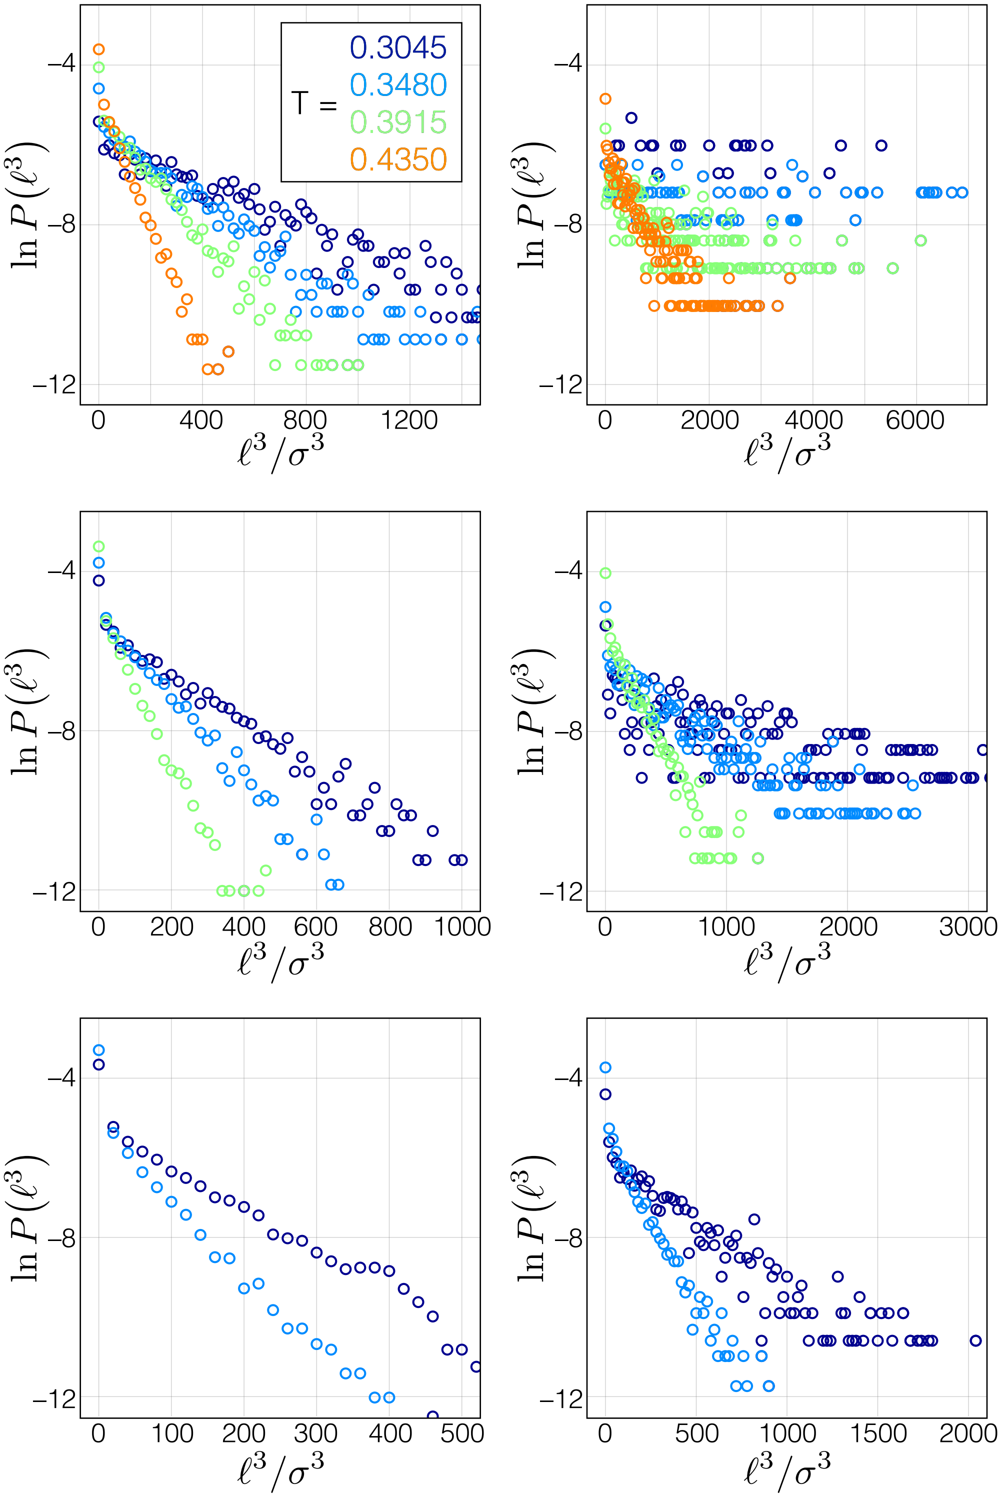


FIG. 1. Distribution of $\ell^3$ for the Kob-Andersen model. Results are shown for the slowest cooling protocol that we performed. For all distributions in this figure, we used the indicator function defined in the main text with a displacement cutoff $a = 0.6\sigma$ (left column) and $1.0\sigma$ (right column), and observation times $t_{\rm obs} = 10\tau_{LJ}$ (top row), $100\tau_{LJ}$ (middle row), and $1000\tau_{LJ}$ (bottom row).

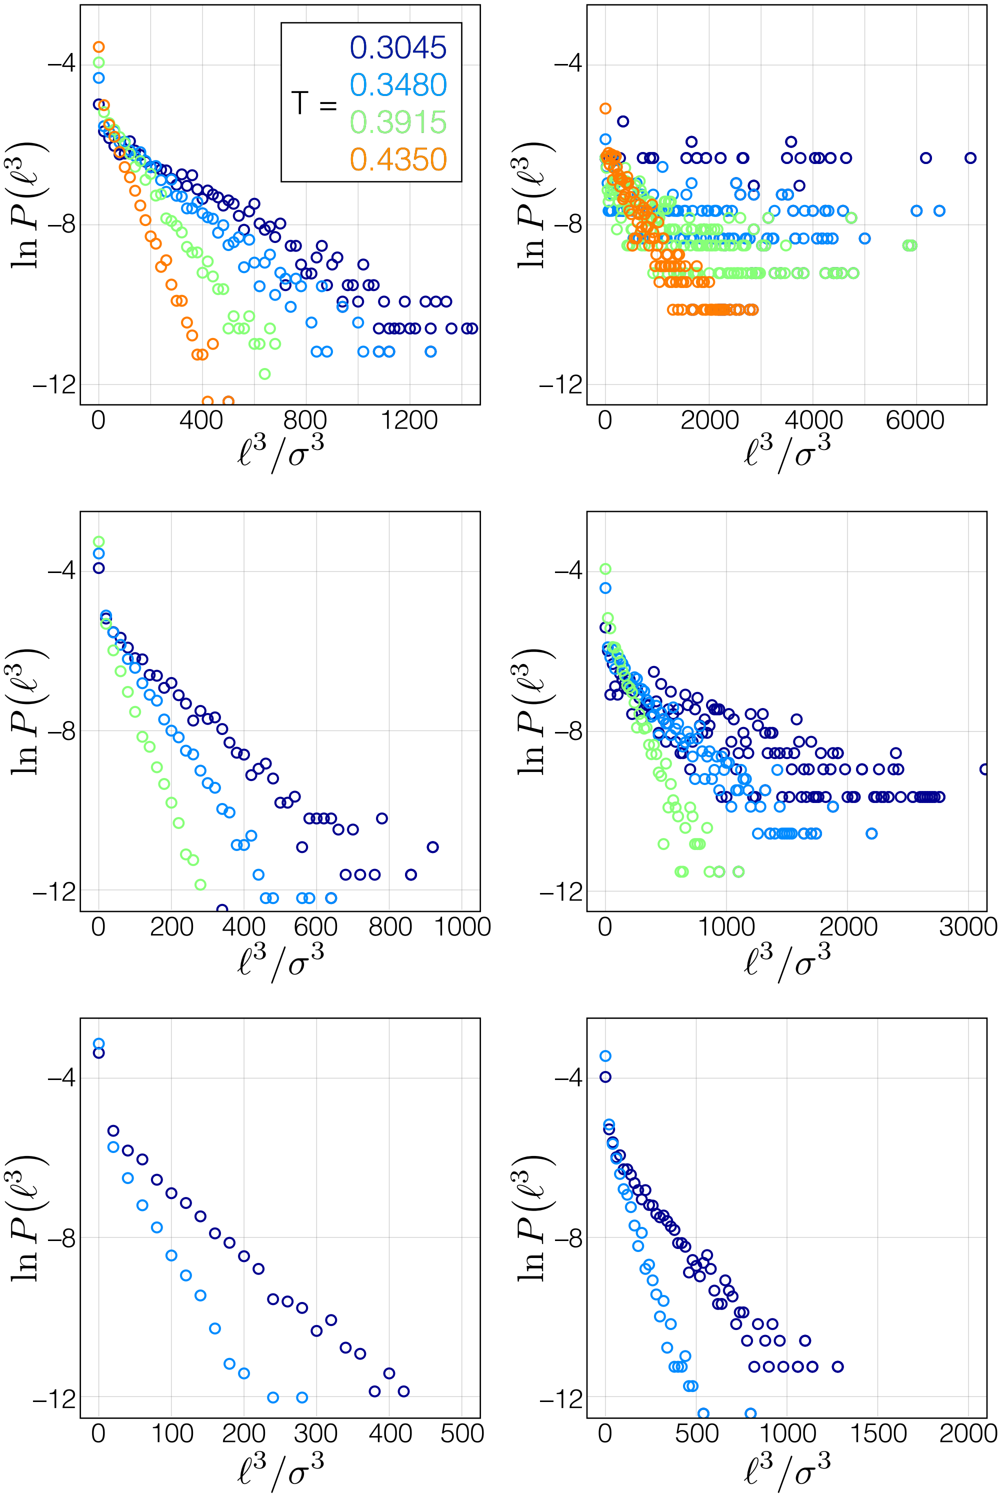


FIG. 2. Distribution of $\ell^3$ for the Kob-Andersen model. Results are shown for the moderate cooling protocol that we performed. For all distributions in this figure, we used the indicator function defined in the main text with a displacement cutoff $a = 0.6\sigma$ (left column) and $1.0\sigma$ (right column), and observation times $t_{\text{obs}} = 10\tau_{LJ}$ (top row), $100\tau_{LJ}$ (middle row), and $1000\tau_{LJ}$ (bottom row).

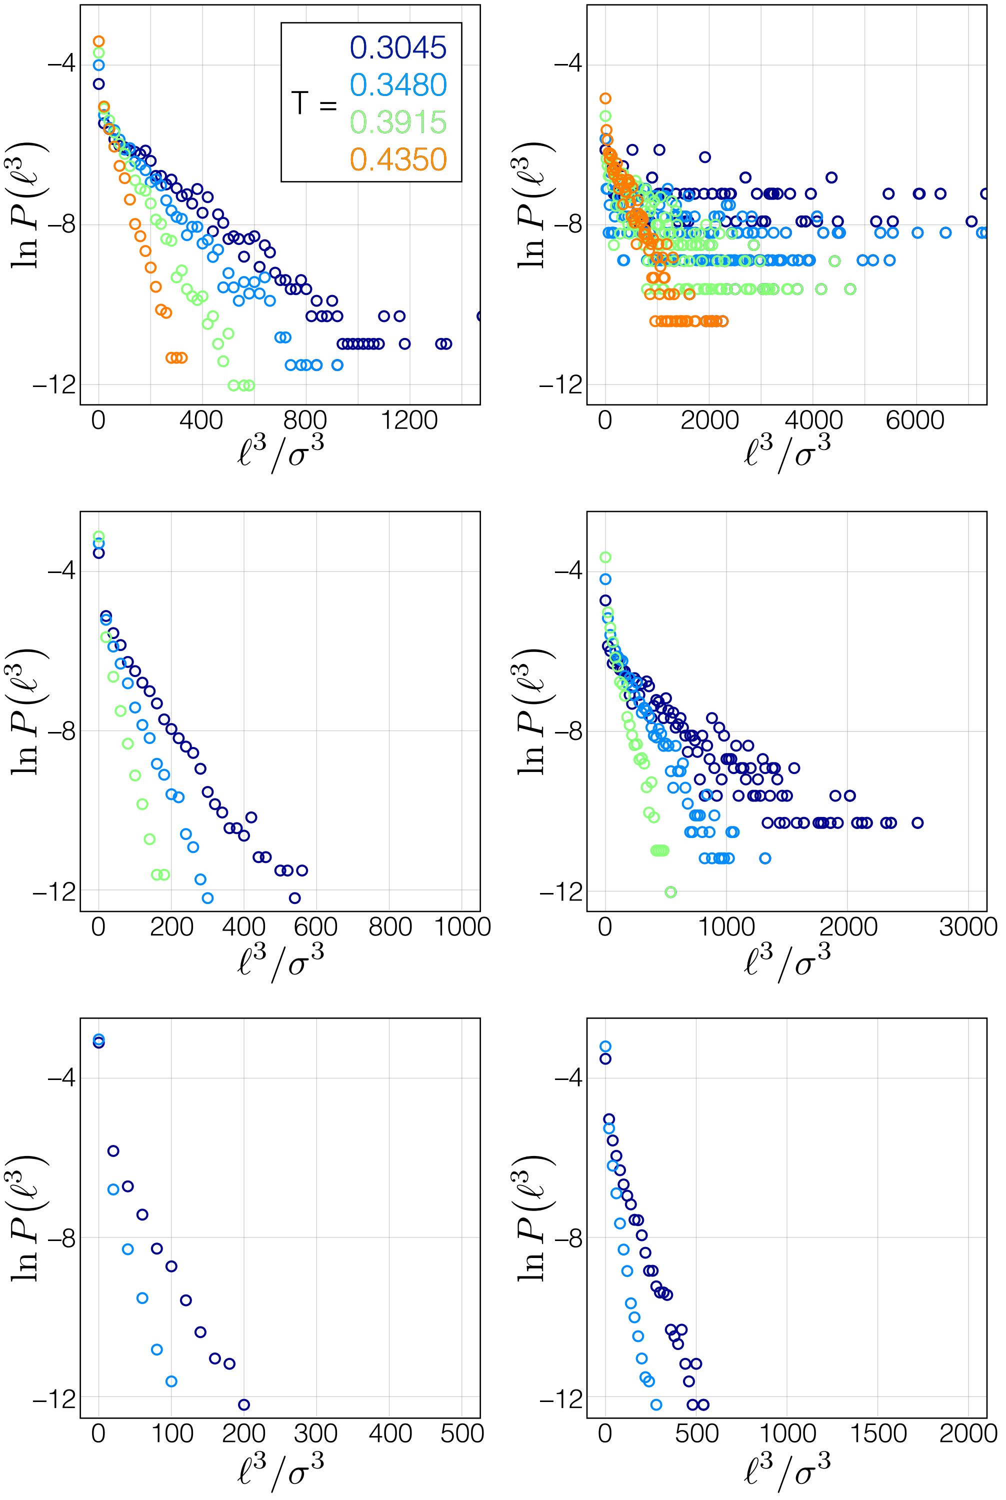


FIG. 3. Distribution of $\ell^3$ for the Kob-Andersen model. Results are shown for the fastest cooling protocol that we performed. For all distributions in this figure, we used the indicator function defined in the main text with a displacement cutoff $a = 0.6\sigma$ (left column) and $1.0\sigma$ (right column), and observation times $t_{\rm obs} = 10\tau_{LJ}$ (top row), $100\tau_{LJ}$ (middle row), and $1000\tau_{LJ}$ (bottom row).

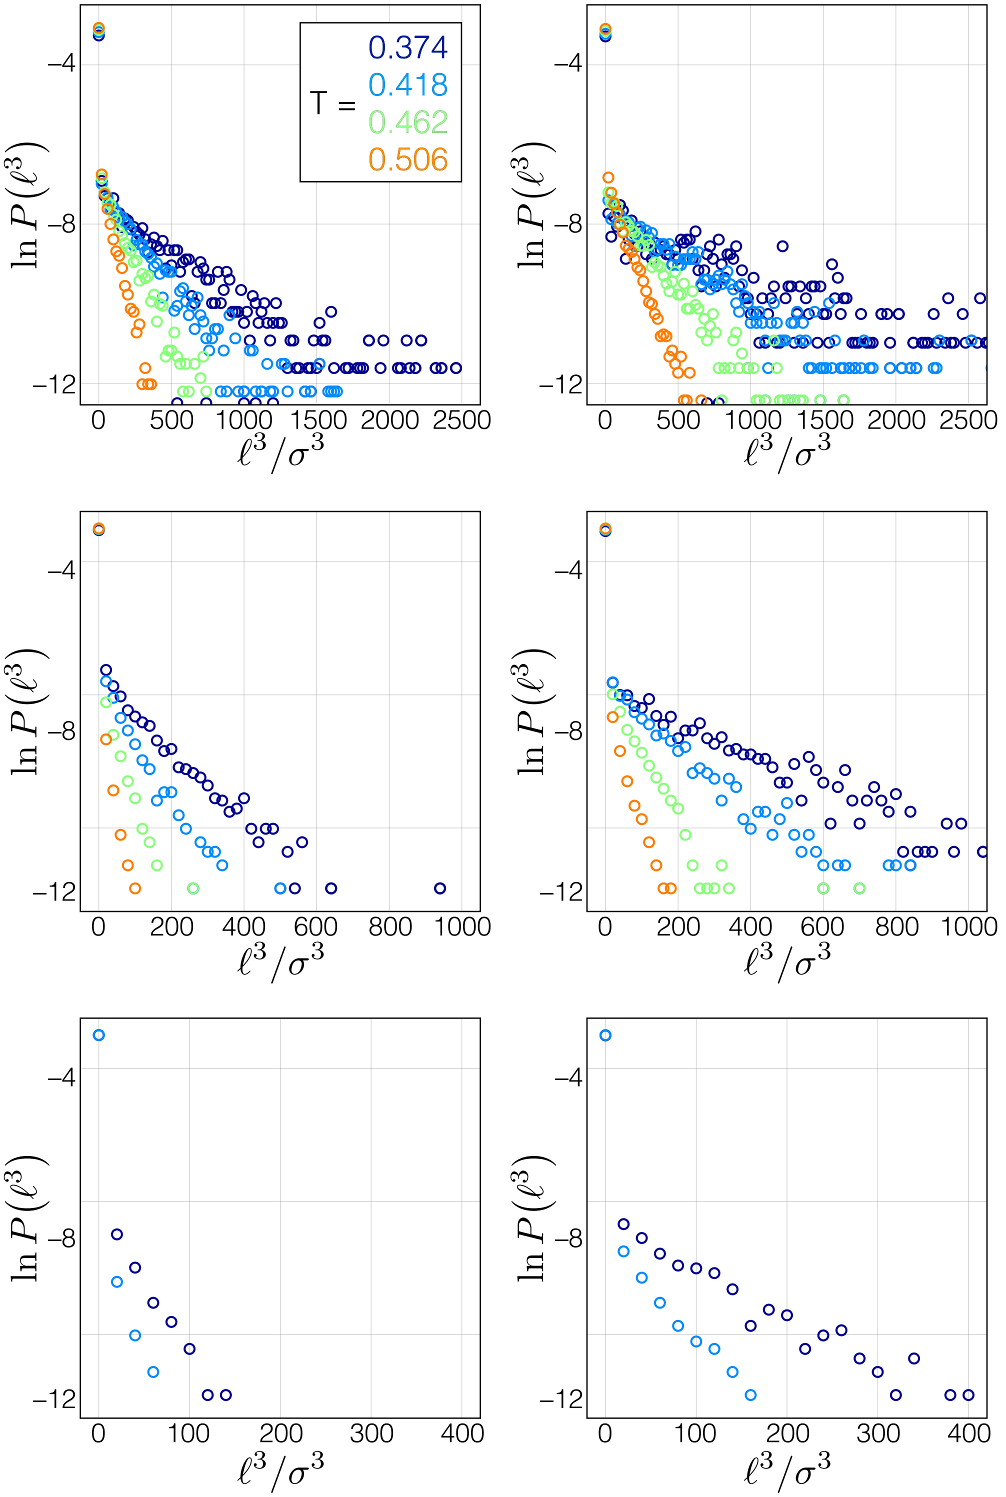


FIG. 4. Distribution of $\ell^3$ for the Wahnström model, for two choices of cooling rate (results of faster cooling shown in the left column, results of slower cooling in the right column). For all distributions in this figure, we used the indicator function defined in the main text with a displacement cutoff $a = 0.6\sigma$, and observation times $t_{\rm obs} = 10\tau_{LJ}$ (top row), $100\tau_{LJ}$ (middle row), and $1000\tau_{LJ}$ (bottom row).

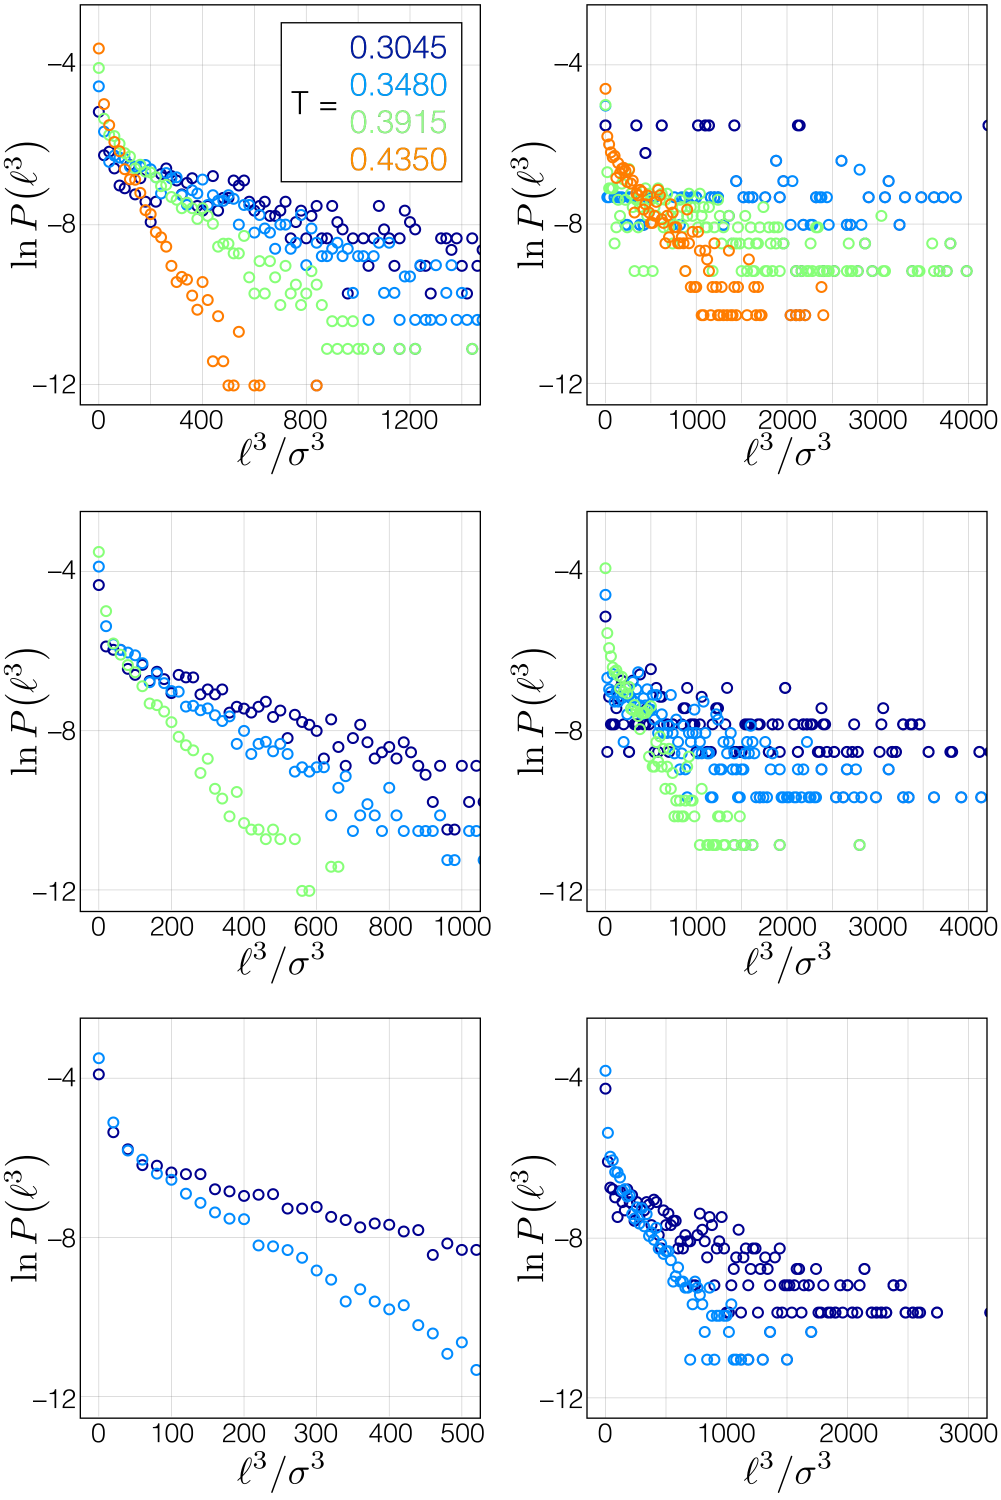


FIG. 5. Distribution of $\ell^3$ for the Kob-Andersen model. Results are shown for the slowest cooling protocol that we performed. For all distributions in this figure, we used an indicator function that selects "strings" of displacing particles as described in the text of this SM, with a replacement cutoff of $a = 0.6$. Results are shown for observation times $t_{\rm obs} = 10\tau_{LJ}$ (top row), $100\tau_{LJ}$ (middle row), and $1000\tau_{LJ}$ (bottom row).
